# Supplementary material for: One Instruction Does Not Fit All: How Well Do Embeddings Align Personas and Instructions in Low-Resource Indian Languages?
Source: arXiv:2601.10205 source file (2026-01-15)
Supplement: Supplementary file 1 [file t2_xling_asm_to_all.tex]

\begin{table*}[t]
\centering
\tiny
\begin{tabular}{lcccccccccccc}
\toprule
\textbf{Model} & \textbf{Ben} & \textbf{Guj} & \textbf{Hin} & \textbf{Kan} & \textbf{Mal} & \textbf{Mar} & \textbf{Odi} & \textbf{Pun} & \textbf{Tam} & \textbf{Tel} & \textbf{Urd} & \textbf{Avg} \\
\midrule
\multicolumn{13}{l}{\textit{Recall@1 (\%)}} \\
multilingual-e5-large-instruct & 22.1 & 18.9 & 21.1 & 19.0 & 17.5 & 20.2 & 18.8 & 17.1 & 15.7 & 17.7 & 19.3 & 18.9 \\
BGE-M3 & 16.5 & 13.7 & 14.7 & 13.7 & 12.6 & 13.3 & 13.2 & 13.0 & 11.5 & 13.3 & 12.8 & 13.5 \\
indic-sentence-bert-nli & 15.2 & 12.2 & 12.6 & 11.9 & 10.7 & 11.6 & 10.2 & 11.9 & 11.6 & 11.5 & 10.6 & 11.8 \\
indic-sentence-similarity-sbert & 11.5 & 9.5 & 10.4 & 10.3 & 8.5 & 9.6 & 7.7 & 10.1 & 9.7 & 9.5 & 9.1 & 9.6 \\
LaBSE & 10.0 & 9.4 & 9.7 & 9.4 & 8.4 & 9.5 & 8.7 & 8.7 & 8.7 & 9.1 & 8.8 & 9.1 \\
\midrule
\multicolumn{13}{l}{\textit{MRR@10}} \\
multilingual-e5-large-instruct & 0.283 & 0.247 & 0.273 & 0.245 & 0.229 & 0.260 & 0.244 & 0.225 & 0.211 & 0.230 & 0.251 & 0.245 \\
BGE-M3 & 0.213 & 0.179 & 0.193 & 0.180 & 0.166 & 0.175 & 0.174 & 0.172 & 0.154 & 0.175 & 0.170 & 0.177 \\
indic-sentence-bert-nli & 0.205 & 0.170 & 0.176 & 0.167 & 0.151 & 0.164 & 0.145 & 0.166 & 0.164 & 0.162 & 0.151 & 0.165 \\
indic-sentence-similarity-sbert & 0.156 & 0.134 & 0.145 & 0.143 & 0.123 & 0.135 & 0.110 & 0.140 & 0.136 & 0.132 & 0.127 & 0.135 \\
LaBSE & 0.138 & 0.131 & 0.134 & 0.131 & 0.117 & 0.131 & 0.121 & 0.121 & 0.123 & 0.128 & 0.123 & 0.127 \\
\bottomrule
\end{tabular}
\caption{Cross-lingual persona$\rightarrow$instruction retrieval (T2) from Assamese to all target languages. Recall@1 (\%) and MRR@10 metrics shown for each source-target pair; averages computed over supported pairs only. Target language abbreviations: Ben=Bengali, Guj=Gujarati, Hin=Hindi, Kan=Kannada, Mal=Malayalam, Mar=Marathi, Odi=Odia, Pun=Punjabi, Tam=Tamil, Tel=Telugu, Urd=Urdu.}
\label{tab:t2_xling_asm}
\end{table*}
