# Supplementary material for: One Instruction Does Not Fit All: How Well Do Embeddings Align Personas and Instructions in Low-Resource Indian Languages?
Source: arXiv:2601.10205 source file (2026-01-15)
Supplement: Supplementary file 2 [file t2_xling_ben_to_all.tex]

\begin{table*}[t]
\centering
\tiny
\begin{tabular}{lcccccccccccc}
\toprule
\textbf{Model} & \textbf{Ass} & \textbf{Guj} & \textbf{Hin} & \textbf{Kan} & \textbf{Mal} & \textbf{Mar} & \textbf{Odi} & \textbf{Pun} & \textbf{Tam} & \textbf{Tel} & \textbf{Urd} & \textbf{Avg} \\
\midrule
\multicolumn{13}{l}{\textit{Recall@1 (\%)}} \\
multilingual-e5-large-instruct & 24.0 & 24.1 & 26.4 & 22.3 & 20.4 & 24.3 & 22.7 & 20.6 & 19.4 & 21.4 & 24.1 & 22.7 \\
BGE-M3 & 16.0 & 15.8 & 17.6 & 16.2 & 14.9 & 15.8 & 14.8 & 15.0 & 13.6 & 15.9 & 15.4 & 15.5 \\
LaBSE & 8.4 & 14.9 & 15.4 & 13.7 & 10.9 & 13.9 & 13.2 & 13.7 & 13.0 & 13.8 & 13.7 & 13.1 \\
indic-sentence-bert-nli & 13.5 & 13.2 & 14.5 & 13.5 & 11.7 & 12.4 & 10.3 & 13.0 & 12.9 & 12.7 & 12.2 & 12.7 \\
indic-sentence-similarity-sbert & 11.0 & 11.4 & 12.7 & 12.3 & 10.0 & 11.3 & 8.1 & 11.7 & 11.5 & 11.0 & 10.4 & 11.0 \\
\midrule
\multicolumn{13}{l}{\textit{MRR@10}} \\
multilingual-e5-large-instruct & 0.304 & 0.306 & 0.333 & 0.285 & 0.265 & 0.308 & 0.289 & 0.267 & 0.255 & 0.276 & 0.306 & 0.290 \\
BGE-M3 & 0.207 & 0.205 & 0.225 & 0.209 & 0.194 & 0.204 & 0.193 & 0.196 & 0.179 & 0.205 & 0.201 & 0.202 \\
LaBSE & 0.115 & 0.195 & 0.201 & 0.181 & 0.147 & 0.182 & 0.175 & 0.180 & 0.172 & 0.181 & 0.181 & 0.174 \\
indic-sentence-bert-nli & 0.186 & 0.183 & 0.200 & 0.186 & 0.165 & 0.175 & 0.147 & 0.180 & 0.179 & 0.176 & 0.171 & 0.177 \\
indic-sentence-similarity-sbert & 0.151 & 0.157 & 0.173 & 0.168 & 0.140 & 0.156 & 0.115 & 0.160 & 0.158 & 0.152 & 0.146 & 0.152 \\
\bottomrule
\end{tabular}
\caption{Cross-lingual persona$\rightarrow$instruction retrieval (T2) from Bengali to all target languages. Recall@1 (\%) and MRR@10 metrics shown for each source-target pair; averages computed over supported pairs only. Target language abbreviations: Ass=Assamese, Guj=Gujarati, Hin=Hindi, Kan=Kannada, Mal=Malayalam, Mar=Marathi, Odi=Odia, Pun=Punjabi, Tam=Tamil, Tel=Telugu, Urd=Urdu.}
\label{tab:t2_xling_ben}
\end{table*}
