# Supplementary material for: One Instruction Does Not Fit All: How Well Do Embeddings Align Personas and Instructions in Low-Resource Indian Languages?
Source: arXiv:2601.10205 source file (2026-01-15)
Supplement: Supplementary file 3 [file t2_xling_guj_to_all.tex]

\begin{table*}[t]
\centering
\tiny
\begin{tabular}{lcccccccccccc}
\toprule
\textbf{Model} & \textbf{Ass} & \textbf{Ben} & \textbf{Hin} & \textbf{Kan} & \textbf{Mal} & \textbf{Mar} & \textbf{Odi} & \textbf{Pun} & \textbf{Tam} & \textbf{Tel} & \textbf{Urd} & \textbf{Avg} \\
\midrule
\multicolumn{13}{l}{\textit{Recall@1 (\%)}} \\
multilingual-e5-large-instruct & 17.5 & 20.7 & 24.0 & 20.9 & 15.3 & 21.0 & 18.9 & 18.8 & 14.9 & 17.6 & 21.0 & 19.2 \\
BGE-M3 & 12.4 & 14.8 & 17.1 & 15.5 & 14.0 & 15.6 & 13.5 & 15.5 & 12.6 & 15.3 & 15.0 & 14.7 \\
LaBSE & 7.5 & 14.3 & 16.8 & 14.8 & 11.5 & 14.8 & 13.6 & 15.0 & 13.7 & 14.8 & 14.9 & 13.8 \\
indic-sentence-bert-nli & 11.2 & 13.4 & 14.7 & 13.4 & 11.4 & 12.6 & 10.3 & 12.7 & 12.5 & 12.7 & 12.3 & 12.5 \\
Para-MPNet & -- & -- & 12.8 & -- & -- & 10.9 & -- & -- & -- & -- & 11.1 & 11.6 \\
indic-sentence-similarity-sbert & 9.2 & 11.4 & 12.1 & 11.6 & 9.5 & 11.0 & 7.7 & 11.5 & 10.6 & 10.6 & 10.2 & 10.5 \\
Para-XLM-R & -- & -- & 8.7 & -- & -- & 8.0 & -- & -- & -- & -- & 7.1 & 7.9 \\
DistilUSE-Multi & -- & -- & 6.2 & -- & -- & 4.3 & -- & -- & -- & -- & 5.1 & 5.2 \\
\midrule
\multicolumn{13}{l}{\textit{MRR@10}} \\
multilingual-e5-large-instruct & 0.228 & 0.266 & 0.304 & 0.267 & 0.201 & 0.268 & 0.243 & 0.246 & 0.198 & 0.230 & 0.269 & 0.247 \\
BGE-M3 & 0.164 & 0.193 & 0.219 & 0.200 & 0.184 & 0.202 & 0.178 & 0.200 & 0.167 & 0.197 & 0.195 & 0.191 \\
LaBSE & 0.104 & 0.185 & 0.216 & 0.190 & 0.152 & 0.191 & 0.179 & 0.194 & 0.180 & 0.191 & 0.194 & 0.180 \\
indic-sentence-bert-nli & 0.160 & 0.186 & 0.202 & 0.185 & 0.161 & 0.177 & 0.149 & 0.180 & 0.174 & 0.176 & 0.174 & 0.175 \\
Para-MPNet & -- & -- & 0.179 & -- & -- & 0.155 & -- & -- & -- & -- & 0.156 & 0.163 \\
indic-sentence-similarity-sbert & 0.129 & 0.157 & 0.165 & 0.159 & 0.133 & 0.150 & 0.110 & 0.157 & 0.147 & 0.147 & 0.143 & 0.145 \\
Para-XLM-R & -- & -- & 0.126 & -- & -- & 0.116 & -- & -- & -- & -- & 0.105 & 0.115 \\
DistilUSE-Multi & -- & -- & 0.089 & -- & -- & 0.063 & -- & -- & -- & -- & 0.076 & 0.076 \\
\bottomrule
\end{tabular}
\caption{Cross-lingual persona$\rightarrow$instruction retrieval (T2) from Gujarati to all target languages. Recall@1 (\%) and MRR@10 metrics shown for each source-target pair; averages computed over supported pairs only. Target language abbreviations: Ass=Assamese, Ben=Bengali, Hin=Hindi, Kan=Kannada, Mal=Malayalam, Mar=Marathi, Odi=Odia, Pun=Punjabi, Tam=Tamil, Tel=Telugu, Urd=Urdu.}
\label{tab:t2_xling_guj}
\end{table*}
