# Supplementary material for: One Instruction Does Not Fit All: How Well Do Embeddings Align Personas and Instructions in Low-Resource Indian Languages?
Source: arXiv:2601.10205 source file (2026-01-15)
Supplement: Supplementary file 4 [file t2_xling_hin_to_all.tex]

\begin{table*}[t]
\centering
\tiny
\begin{tabular}{lcccccccccccc}
\toprule
\textbf{Model} & \textbf{Ass} & \textbf{Ben} & \textbf{Guj} & \textbf{Kan} & \textbf{Mal} & \textbf{Mar} & \textbf{Odi} & \textbf{Pun} & \textbf{Tam} & \textbf{Tel} & \textbf{Urd} & \textbf{Avg} \\
\midrule
\multicolumn{13}{l}{\textit{Recall@1 (\%)}} \\
multilingual-e5-large-instruct & 19.9 & 24.6 & 23.0 & 24.9 & 17.0 & 27.5 & 21.5 & 20.2 & 18.3 & 21.6 & 23.2 & 22.0 \\
Para-MPNet & -- & -- & 13.2 & -- & -- & 16.5 & -- & -- & -- & -- & 14.8 & 14.9 \\
BGE-M3 & 11.9 & 14.6 & 15.6 & 15.2 & 13.6 & 18.4 & 13.0 & 14.8 & 12.4 & 14.8 & 15.2 & 14.5 \\
LaBSE & 7.5 & 14.4 & 16.8 & 14.9 & 11.3 & 15.9 & 13.9 & 15.3 & 14.1 & 14.9 & 15.4 & 14.0 \\
indic-sentence-bert-nli & 12.3 & 14.8 & 14.7 & 14.9 & 12.4 & 15.6 & 11.1 & 14.8 & 14.0 & 13.7 & 10.3 & 13.5 \\
indic-sentence-similarity-sbert & 10.1 & 12.9 & 12.3 & 13.1 & 10.3 & 13.3 & 8.2 & 12.6 & 12.0 & 11.5 & 11.2 & 11.6 \\
Para-XLM-R & -- & -- & 9.1 & -- & -- & 11.7 & -- & -- & -- & -- & 9.4 & 10.1 \\
DistilUSE-Multi & -- & -- & 5.9 & -- & -- & 9.3 & -- & -- & -- & -- & 9.7 & 8.3 \\
\midrule
\multicolumn{13}{l}{\textit{MRR@10}} \\
multilingual-e5-large-instruct & 0.264 & 0.316 & 0.298 & 0.319 & 0.230 & 0.346 & 0.280 & 0.270 & 0.247 & 0.282 & 0.301 & 0.286 \\
Para-MPNet & -- & -- & 0.183 & -- & -- & 0.222 & -- & -- & -- & -- & 0.202 & 0.202 \\
BGE-M3 & 0.160 & 0.192 & 0.202 & 0.198 & 0.180 & 0.234 & 0.173 & 0.193 & 0.165 & 0.193 & 0.199 & 0.190 \\
LaBSE & 0.103 & 0.187 & 0.215 & 0.193 & 0.150 & 0.203 & 0.181 & 0.197 & 0.184 & 0.192 & 0.199 & 0.182 \\
indic-sentence-bert-nli & 0.174 & 0.203 & 0.201 & 0.204 & 0.173 & 0.211 & 0.157 & 0.202 & 0.192 & 0.189 & 0.149 & 0.187 \\
indic-sentence-similarity-sbert & 0.141 & 0.176 & 0.167 & 0.177 & 0.144 & 0.179 & 0.116 & 0.171 & 0.163 & 0.158 & 0.154 & 0.159 \\
Para-XLM-R & -- & -- & 0.132 & -- & -- & 0.163 & -- & -- & -- & -- & 0.136 & 0.144 \\
DistilUSE-Multi & -- & -- & 0.085 & -- & -- & 0.128 & -- & -- & -- & -- & 0.136 & 0.116 \\
\bottomrule
\end{tabular}
\caption{Cross-lingual persona$\rightarrow$instruction retrieval (T2) from Hindi to all target languages. Recall@1 (\%) and MRR@10 metrics shown for each source-target pair; averages computed over supported pairs only. Target language abbreviations: Ass=Assamese, Ben=Bengali, Guj=Gujarati, Kan=Kannada, Mal=Malayalam, Mar=Marathi, Odi=Odia, Pun=Punjabi, Tam=Tamil, Tel=Telugu, Urd=Urdu.}
\label{tab:t2_xling_hin}
\end{table*}
