# Supplementary material for: One Instruction Does Not Fit All: How Well Do Embeddings Align Personas and Instructions in Low-Resource Indian Languages?
Source: arXiv:2601.10205 source file (2026-01-15)
Supplement: Supplementary file 5 [file t2_xling_kan_to_all.tex]

\begin{table*}[t]
\centering
\tiny
\begin{tabular}{lcccccccccccc}
\toprule
\textbf{Model} & \textbf{Ass} & \textbf{Ben} & \textbf{Guj} & \textbf{Hin} & \textbf{Mal} & \textbf{Mar} & \textbf{Odi} & \textbf{Pun} & \textbf{Tam} & \textbf{Tel} & \textbf{Urd} & \textbf{Avg} \\
\midrule
\multicolumn{13}{l}{\textit{Recall@1 (\%)}} \\
multilingual-e5-large-instruct & 16.6 & 20.1 & 22.0 & 26.0 & 20.0 & 22.6 & 20.4 & 20.4 & 18.3 & 21.6 & 22.8 & 21.0 \\
BGE-M3 & 13.2 & 15.8 & 16.4 & 17.9 & 16.0 & 16.4 & 14.7 & 15.6 & 15.0 & 17.8 & 16.0 & 15.9 \\
LaBSE & 8.4 & 14.8 & 16.4 & 17.0 & 12.5 & 15.3 & 14.1 & 15.1 & 14.7 & 15.6 & 15.1 & 14.4 \\
indic-sentence-bert-nli & 12.8 & 14.8 & 14.5 & 15.7 & 13.2 & 13.9 & 11.3 & 14.6 & 14.7 & 14.5 & 13.4 & 13.9 \\
indic-sentence-similarity-sbert & 9.6 & 11.8 & 11.1 & 12.4 & 10.1 & 11.2 & 7.9 & 11.5 & 11.7 & 11.5 & 10.3 & 10.8 \\
\midrule
\multicolumn{13}{l}{\textit{MRR@10}} \\
multilingual-e5-large-instruct & 0.217 & 0.259 & 0.281 & 0.327 & 0.255 & 0.286 & 0.261 & 0.264 & 0.238 & 0.274 & 0.291 & 0.268 \\
BGE-M3 & 0.173 & 0.205 & 0.211 & 0.227 & 0.207 & 0.210 & 0.190 & 0.201 & 0.195 & 0.225 & 0.207 & 0.205 \\
LaBSE & 0.114 & 0.193 & 0.212 & 0.218 & 0.165 & 0.199 & 0.184 & 0.195 & 0.193 & 0.203 & 0.197 & 0.188 \\
indic-sentence-bert-nli & 0.179 & 0.202 & 0.198 & 0.214 & 0.183 & 0.192 & 0.159 & 0.198 & 0.200 & 0.197 & 0.185 & 0.192 \\
indic-sentence-similarity-sbert & 0.134 & 0.162 & 0.153 & 0.168 & 0.141 & 0.154 & 0.112 & 0.157 & 0.159 & 0.157 & 0.143 & 0.149 \\
\bottomrule
\end{tabular}
\caption{Cross-lingual persona$\rightarrow$instruction retrieval (T2) from Kannada to all target languages. Recall@1 (\%) and MRR@10 metrics shown for each source-target pair; averages computed over supported pairs only. Target language abbreviations: Ass=Assamese, Ben=Bengali, Guj=Gujarati, Hin=Hindi, Mal=Malayalam, Mar=Marathi, Odi=Odia, Pun=Punjabi, Tam=Tamil, Tel=Telugu, Urd=Urdu.}
\label{tab:t2_xling_kan}
\end{table*}
