# Supplementary material for: One Instruction Does Not Fit All: How Well Do Embeddings Align Personas and Instructions in Low-Resource Indian Languages?
Source: arXiv:2601.10205 source file (2026-01-15)
Supplement: Supplementary file 6 [file t2_xling_mal_to_all.tex]

\begin{table*}[t]
\centering
\tiny
\begin{tabular}{lcccccccccccc}
\toprule
\textbf{Model} & \textbf{Ass} & \textbf{Ben} & \textbf{Guj} & \textbf{Hin} & \textbf{Kan} & \textbf{Mar} & \textbf{Odi} & \textbf{Pun} & \textbf{Tam} & \textbf{Tel} & \textbf{Urd} & \textbf{Avg} \\
\midrule
\multicolumn{13}{l}{\textit{Recall@1 (\%)}} \\
multilingual-e5-large-instruct & 18.4 & 21.3 & 21.3 & 24.4 & 22.4 & 21.5 & 18.8 & 19.1 & 18.0 & 20.2 & 22.7 & 20.7 \\
BGE-M3 & 12.0 & 14.8 & 15.2 & 16.4 & 16.3 & 14.8 & 13.3 & 14.5 & 14.1 & 16.0 & 15.0 & 14.8 \\
LaBSE & 7.8 & 12.5 & 13.6 & 14.1 & 13.4 & 13.0 & 11.9 & 12.7 & 12.7 & 13.4 & 12.9 & 12.5 \\
indic-sentence-bert-nli & 11.2 & 13.1 & 12.8 & 13.7 & 13.6 & 12.2 & 10.0 & 13.0 & 13.5 & 13.0 & 11.8 & 12.5 \\
indic-sentence-similarity-sbert & 8.3 & 10.2 & 9.5 & 10.3 & 10.5 & 9.5 & 7.2 & 10.1 & 10.0 & 9.9 & 8.8 & 9.5 \\
\midrule
\multicolumn{13}{l}{\textit{MRR@10}} \\
multilingual-e5-large-instruct & 0.240 & 0.275 & 0.274 & 0.310 & 0.286 & 0.276 & 0.245 & 0.251 & 0.238 & 0.260 & 0.290 & 0.268 \\
BGE-M3 & 0.161 & 0.193 & 0.197 & 0.210 & 0.209 & 0.193 & 0.176 & 0.189 & 0.185 & 0.206 & 0.197 & 0.192 \\
LaBSE & 0.106 & 0.167 & 0.181 & 0.185 & 0.177 & 0.172 & 0.159 & 0.168 & 0.168 & 0.177 & 0.171 & 0.166 \\
indic-sentence-bert-nli & 0.160 & 0.181 & 0.178 & 0.189 & 0.186 & 0.171 & 0.144 & 0.180 & 0.186 & 0.179 & 0.167 & 0.175 \\
indic-sentence-similarity-sbert & 0.119 & 0.142 & 0.134 & 0.144 & 0.145 & 0.133 & 0.103 & 0.140 & 0.140 & 0.138 & 0.126 & 0.133 \\
\bottomrule
\end{tabular}
\caption{Cross-lingual persona$\rightarrow$instruction retrieval (T2) from Malayalam to all target languages. Recall@1 (\%) and MRR@10 metrics shown for each source-target pair; averages computed over supported pairs only. Target language abbreviations: Ass=Assamese, Ben=Bengali, Guj=Gujarati, Hin=Hindi, Kan=Kannada, Mar=Marathi, Odi=Odia, Pun=Punjabi, Tam=Tamil, Tel=Telugu, Urd=Urdu.}
\label{tab:t2_xling_mal}
\end{table*}
