# Supplementary material for: One Instruction Does Not Fit All: How Well Do Embeddings Align Personas and Instructions in Low-Resource Indian Languages?
Source: arXiv:2601.10205 source file (2026-01-15)
Supplement: Supplementary file 7 [file t2_xling_mar_to_all.tex]

\begin{table*}[t]
\centering
\tiny
\begin{tabular}{lcccccccccccc}
\toprule
\textbf{Model} & \textbf{Ass} & \textbf{Ben} & \textbf{Guj} & \textbf{Hin} & \textbf{Kan} & \textbf{Mal} & \textbf{Odi} & \textbf{Pun} & \textbf{Tam} & \textbf{Tel} & \textbf{Urd} & \textbf{Avg} \\
\midrule
\multicolumn{13}{l}{\textit{Recall@1 (\%)}} \\
multilingual-e5-large-instruct & 18.8 & 23.0 & 21.4 & 28.3 & 22.8 & 17.5 & 19.5 & 19.0 & 18.0 & 20.7 & 22.3 & 21.0 \\
BGE-M3 & 13.0 & 16.1 & 16.9 & 21.7 & 16.7 & 15.1 & 14.4 & 15.6 & 14.0 & 16.3 & 16.1 & 16.0 \\
Para-MPNet & -- & -- & 11.7 & 17.4 & -- & -- & -- & -- & -- & -- & 12.9 & 14.0 \\
LaBSE & 8.2 & 14.2 & 16.0 & 17.3 & 14.8 & 11.7 & 13.5 & 14.5 & 14.0 & 14.7 & 14.5 & 13.9 \\
indic-sentence-bert-nli & 9.8 & 13.3 & 12.9 & 13.6 & 12.3 & 8.2 & 9.8 & 12.9 & 9.0 & 10.4 & 10.1 & 11.1 \\
indic-sentence-similarity-sbert & 9.3 & 11.6 & 11.0 & 13.4 & 11.6 & 9.6 & 7.7 & 11.3 & 10.8 & 10.7 & 10.0 & 10.6 \\
Para-XLM-R & -- & -- & 7.4 & 10.5 & -- & -- & -- & -- & -- & -- & 7.8 & 8.6 \\
DistilUSE-Multi & -- & -- & 4.6 & 10.3 & -- & -- & -- & -- & -- & -- & 7.1 & 7.3 \\
\midrule
\multicolumn{13}{l}{\textit{MRR@10}} \\
multilingual-e5-large-instruct & 0.247 & 0.294 & 0.278 & 0.352 & 0.292 & 0.233 & 0.255 & 0.251 & 0.239 & 0.269 & 0.287 & 0.272 \\
BGE-M3 & 0.173 & 0.209 & 0.219 & 0.270 & 0.215 & 0.196 & 0.188 & 0.203 & 0.183 & 0.210 & 0.209 & 0.207 \\
Para-MPNet & -- & -- & 0.165 & 0.232 & -- & -- & -- & -- & -- & -- & 0.180 & 0.192 \\
LaBSE & 0.111 & 0.186 & 0.207 & 0.222 & 0.192 & 0.156 & 0.178 & 0.189 & 0.183 & 0.193 & 0.191 & 0.182 \\
indic-sentence-bert-nli & 0.146 & 0.186 & 0.181 & 0.196 & 0.177 & 0.139 & 0.141 & 0.180 & 0.152 & 0.159 & 0.153 & 0.165 \\
indic-sentence-similarity-sbert & 0.130 & 0.159 & 0.152 & 0.180 & 0.159 & 0.134 & 0.109 & 0.154 & 0.149 & 0.146 & 0.139 & 0.147 \\
Para-XLM-R & -- & -- & 0.107 & 0.147 & -- & -- & -- & -- & -- & -- & 0.111 & 0.122 \\
DistilUSE-Multi & -- & -- & 0.067 & 0.144 & -- & -- & -- & -- & -- & -- & 0.104 & 0.105 \\
\bottomrule
\end{tabular}
\caption{Cross-lingual persona$\rightarrow$instruction retrieval (T2) from Marathi to all target languages. Recall@1 (\%) and MRR@10 metrics shown for each source-target pair; averages computed over supported pairs only. Target language abbreviations: Ass=Assamese, Ben=Bengali, Guj=Gujarati, Hin=Hindi, Kan=Kannada, Mal=Malayalam, Odi=Odia, Pun=Punjabi, Tam=Tamil, Tel=Telugu, Urd=Urdu.}
\label{tab:t2_xling_mar}
\end{table*}
