# Supplementary material for: One Instruction Does Not Fit All: How Well Do Embeddings Align Personas and Instructions in Low-Resource Indian Languages?
Source: arXiv:2601.10205 source file (2026-01-15)
Supplement: Supplementary file 8 [file t2_xling_ory_to_all.tex]

\begin{table*}[t]
\centering
\tiny
\begin{tabular}{lcccccccccccc}
\toprule
\textbf{Model} & \textbf{Ass} & \textbf{Ben} & \textbf{Guj} & \textbf{Hin} & \textbf{Kan} & \textbf{Mal} & \textbf{Mar} & \textbf{Pun} & \textbf{Tam} & \textbf{Tel} & \textbf{Urd} & \textbf{Avg} \\
\midrule
\multicolumn{13}{l}{\textit{Recall@1 (\%)}} \\
multilingual-e5-large-instruct & 18.3 & 21.4 & 20.3 & 22.3 & 20.4 & 16.9 & 19.9 & 18.1 & 12.7 & 18.7 & 20.1 & 19.0 \\
BGE-M3 & 11.9 & 14.0 & 14.1 & 15.0 & 14.0 & 12.6 & 13.5 & 13.5 & 11.5 & 13.8 & 13.0 & 13.4 \\
LaBSE & 8.1 & 13.6 & 14.2 & 14.6 & 13.3 & 10.7 & 13.4 & 13.2 & 12.3 & 13.1 & 13.2 & 12.7 \\
indic-sentence-bert-nli & 5.8 & 12.1 & 11.9 & 12.4 & 11.8 & 10.4 & 10.8 & 11.7 & 11.4 & 11.5 & 10.7 & 11.0 \\
indic-sentence-similarity-sbert & 6.9 & 8.7 & 8.3 & 8.7 & 8.7 & 7.5 & 8.2 & 8.7 & 7.9 & 8.2 & 7.4 & 8.1 \\
\midrule
\multicolumn{13}{l}{\textit{MRR@10}} \\
multilingual-e5-large-instruct & 0.237 & 0.272 & 0.261 & 0.286 & 0.261 & 0.221 & 0.255 & 0.236 & 0.171 & 0.242 & 0.258 & 0.246 \\
BGE-M3 & 0.160 & 0.184 & 0.185 & 0.195 & 0.184 & 0.168 & 0.178 & 0.178 & 0.155 & 0.180 & 0.173 & 0.176 \\
LaBSE & 0.111 & 0.177 & 0.187 & 0.192 & 0.175 & 0.144 & 0.176 & 0.174 & 0.165 & 0.174 & 0.174 & 0.168 \\
indic-sentence-bert-nli & 0.094 & 0.169 & 0.167 & 0.173 & 0.166 & 0.148 & 0.154 & 0.165 & 0.161 & 0.161 & 0.152 & 0.156 \\
indic-sentence-similarity-sbert & 0.100 & 0.122 & 0.117 & 0.124 & 0.122 & 0.109 & 0.117 & 0.122 & 0.115 & 0.118 & 0.107 & 0.116 \\
\bottomrule
\end{tabular}
\caption{Cross-lingual persona$\rightarrow$instruction retrieval (T2) from Odia to all target languages. Recall@1 (\%) and MRR@10 metrics shown for each source-target pair; averages computed over supported pairs only. Target language abbreviations: Ass=Assamese, Ben=Bengali, Guj=Gujarati, Hin=Hindi, Kan=Kannada, Mal=Malayalam, Mar=Marathi, Pun=Punjabi, Tam=Tamil, Tel=Telugu, Urd=Urdu.}
\label{tab:t2_xling_ory}
\end{table*}
