# Supplementary material for: One Instruction Does Not Fit All: How Well Do Embeddings Align Personas and Instructions in Low-Resource Indian Languages?
Source: arXiv:2601.10205 source file (2026-01-15)
Supplement: Supplementary file 9 [file t2_xling_pan_to_all.tex]

\begin{table*}[t]
\centering
\tiny
\begin{tabular}{lcccccccccccc}
\toprule
\textbf{Model} & \textbf{Ass} & \textbf{Ben} & \textbf{Guj} & \textbf{Hin} & \textbf{Kan} & \textbf{Mal} & \textbf{Mar} & \textbf{Odi} & \textbf{Tam} & \textbf{Tel} & \textbf{Urd} & \textbf{Avg} \\
\midrule
\multicolumn{13}{l}{\textit{Recall@1 (\%)}} \\
multilingual-e5-large-instruct & 19.1 & 22.6 & 23.7 & 25.2 & 22.3 & 18.4 & 22.3 & 20.8 & 17.0 & 18.4 & 23.8 & 21.2 \\
LaBSE & 7.8 & 13.2 & 14.8 & 15.4 & 13.8 & 11.3 & 13.6 & 12.8 & 12.8 & 13.6 & 14.1 & 13.0 \\
indic-sentence-bert-nli & 11.4 & 14.0 & 14.1 & 15.6 & 14.1 & 12.1 & 13.1 & 11.0 & 13.4 & 13.3 & 8.1 & 12.8 \\
BGE-M3 & 10.4 & 12.2 & 13.6 & 14.4 & 13.0 & 11.5 & 12.6 & 11.5 & 10.3 & 12.6 & 13.2 & 12.3 \\
indic-sentence-similarity-sbert & 9.4 & 11.7 & 11.4 & 12.6 & 11.9 & 9.9 & 11.2 & 8.1 & 11.1 & 11.0 & 10.6 & 10.8 \\
\midrule
\multicolumn{13}{l}{\textit{MRR@10}} \\
multilingual-e5-large-instruct & 0.247 & 0.289 & 0.301 & 0.318 & 0.285 & 0.239 & 0.283 & 0.267 & 0.224 & 0.239 & 0.301 & 0.272 \\
LaBSE & 0.107 & 0.174 & 0.195 & 0.201 & 0.181 & 0.150 & 0.179 & 0.170 & 0.169 & 0.179 & 0.185 & 0.172 \\
indic-sentence-bert-nli & 0.164 & 0.194 & 0.195 & 0.211 & 0.194 & 0.171 & 0.184 & 0.157 & 0.185 & 0.184 & 0.120 & 0.178 \\
BGE-M3 & 0.141 & 0.163 & 0.178 & 0.188 & 0.171 & 0.155 & 0.166 & 0.154 & 0.141 & 0.167 & 0.175 & 0.164 \\
indic-sentence-similarity-sbert & 0.133 & 0.162 & 0.157 & 0.171 & 0.162 & 0.138 & 0.153 & 0.115 & 0.152 & 0.151 & 0.147 & 0.149 \\
\bottomrule
\end{tabular}
\caption{Cross-lingual persona$\rightarrow$instruction retrieval (T2) from Punjabi to all target languages. Recall@1 (\%) and MRR@10 metrics shown for each source-target pair; averages computed over supported pairs only. Target language abbreviations: Ass=Assamese, Ben=Bengali, Guj=Gujarati, Hin=Hindi, Kan=Kannada, Mal=Malayalam, Mar=Marathi, Odi=Odia, Tam=Tamil, Tel=Telugu, Urd=Urdu.}
\label{tab:t2_xling_pan}
\end{table*}
