# Supplementary material for: One Instruction Does Not Fit All: How Well Do Embeddings Align Personas and Instructions in Low-Resource Indian Languages?
Source: arXiv:2601.10205 source file (2026-01-15)
Supplement: Supplementary file 10 [file t2_xling_tam_to_all.tex]

\begin{table*}[t]
\centering
\tiny
\begin{tabular}{lcccccccccccc}
\toprule
\textbf{Model} & \textbf{Ass} & \textbf{Ben} & \textbf{Guj} & \textbf{Hin} & \textbf{Kan} & \textbf{Mal} & \textbf{Mar} & \textbf{Odi} & \textbf{Pun} & \textbf{Tel} & \textbf{Urd} & \textbf{Avg} \\
\midrule
\multicolumn{13}{l}{\textit{Recall@1 (\%)}} \\
multilingual-e5-large-instruct & 17.9 & 20.4 & 20.6 & 24.0 & 21.7 & 17.9 & 21.8 & 17.7 & 18.7 & 19.6 & 21.6 & 20.2 \\
LaBSE & 7.8 & 13.5 & 15.2 & 15.8 & 14.5 & 11.8 & 14.2 & 13.0 & 13.9 & 14.4 & 14.1 & 13.5 \\
BGE-M3 & 10.6 & 12.5 & 12.9 & 14.4 & 14.3 & 13.4 & 13.2 & 11.5 & 12.5 & 14.0 & 13.2 & 13.0 \\
indic-sentence-bert-nli & 10.8 & 12.3 & 11.9 & 13.5 & 13.2 & 11.2 & 11.5 & 9.3 & 12.3 & 12.1 & 11.7 & 11.8 \\
indic-sentence-similarity-sbert & 8.8 & 11.1 & 10.1 & 11.4 & 11.6 & 9.6 & 10.2 & 7.2 & 10.5 & 10.6 & 9.5 & 10.1 \\
\midrule
\multicolumn{13}{l}{\textit{MRR@10}} \\
multilingual-e5-large-instruct & 0.232 & 0.263 & 0.267 & 0.306 & 0.276 & 0.234 & 0.279 & 0.231 & 0.243 & 0.253 & 0.278 & 0.260 \\
LaBSE & 0.106 & 0.178 & 0.197 & 0.205 & 0.189 & 0.156 & 0.185 & 0.172 & 0.182 & 0.188 & 0.186 & 0.177 \\
BGE-M3 & 0.142 & 0.166 & 0.170 & 0.187 & 0.186 & 0.176 & 0.172 & 0.153 & 0.165 & 0.182 & 0.175 & 0.170 \\
indic-sentence-bert-nli & 0.156 & 0.175 & 0.171 & 0.190 & 0.185 & 0.161 & 0.166 & 0.138 & 0.173 & 0.172 & 0.165 & 0.169 \\
indic-sentence-similarity-sbert & 0.125 & 0.153 & 0.141 & 0.156 & 0.159 & 0.135 & 0.142 & 0.104 & 0.146 & 0.146 & 0.134 & 0.140 \\
\bottomrule
\end{tabular}
\caption{Cross-lingual persona$\rightarrow$instruction retrieval (T2) from Tamil to all target languages. Recall@1 (\%) and MRR@10 metrics shown for each source-target pair; averages computed over supported pairs only. Target language abbreviations: Ass=Assamese, Ben=Bengali, Guj=Gujarati, Hin=Hindi, Kan=Kannada, Mal=Malayalam, Mar=Marathi, Odi=Odia, Pun=Punjabi, Tel=Telugu, Urd=Urdu.}
\label{tab:t2_xling_tam}
\end{table*}
