# Supplementary material for: One Instruction Does Not Fit All: How Well Do Embeddings Align Personas and Instructions in Low-Resource Indian Languages?
Source: arXiv:2601.10205 source file (2026-01-15)
Supplement: Supplementary file 11 [file t2_xling_tel_to_all.tex]

\begin{table*}[t]
\centering
\tiny
\begin{tabular}{lcccccccccccc}
\toprule
\textbf{Model} & \textbf{Ass} & \textbf{Ben} & \textbf{Guj} & \textbf{Hin} & \textbf{Kan} & \textbf{Mal} & \textbf{Mar} & \textbf{Odi} & \textbf{Pun} & \textbf{Tam} & \textbf{Urd} & \textbf{Avg} \\
\midrule
\multicolumn{13}{l}{\textit{Recall@1 (\%)}} \\
multilingual-e5-large-instruct & 17.6 & 21.1 & 20.8 & 24.7 & 23.1 & 18.4 & 23.0 & 19.6 & 17.4 & 17.7 & 21.7 & 20.5 \\
BGE-M3 & 13.2 & 16.0 & 16.5 & 17.9 & 18.1 & 16.4 & 16.4 & 14.7 & 15.8 & 14.7 & 16.3 & 16.0 \\
LaBSE & 8.3 & 14.6 & 16.6 & 17.1 & 15.8 & 12.8 & 15.4 & 14.1 & 15.2 & 14.8 & 15.4 & 14.6 \\
indic-sentence-bert-nli & 10.8 & 13.8 & 14.1 & 14.8 & 14.4 & 12.6 & 13.2 & 11.2 & 13.8 & 14.0 & 12.3 & 13.2 \\
indic-sentence-similarity-sbert & 9.1 & 11.2 & 10.6 & 11.5 & 11.9 & 9.9 & 10.5 & 7.7 & 11.0 & 11.2 & 10.1 & 10.4 \\
\midrule
\multicolumn{13}{l}{\textit{MRR@10}} \\
multilingual-e5-large-instruct & 0.231 & 0.270 & 0.268 & 0.314 & 0.293 & 0.238 & 0.293 & 0.254 & 0.230 & 0.234 & 0.279 & 0.264 \\
BGE-M3 & 0.173 & 0.207 & 0.213 & 0.229 & 0.230 & 0.211 & 0.211 & 0.191 & 0.204 & 0.193 & 0.211 & 0.206 \\
LaBSE & 0.113 & 0.192 & 0.214 & 0.220 & 0.205 & 0.168 & 0.200 & 0.185 & 0.196 & 0.193 & 0.200 & 0.190 \\
indic-sentence-bert-nli & 0.155 & 0.190 & 0.192 & 0.202 & 0.196 & 0.175 & 0.183 & 0.157 & 0.191 & 0.192 & 0.171 & 0.182 \\
indic-sentence-similarity-sbert & 0.127 & 0.154 & 0.147 & 0.158 & 0.162 & 0.138 & 0.146 & 0.110 & 0.151 & 0.153 & 0.139 & 0.144 \\
\bottomrule
\end{tabular}
\caption{Cross-lingual persona$\rightarrow$instruction retrieval (T2) from Telugu to all target languages. Recall@1 (\%) and MRR@10 metrics shown for each source-target pair; averages computed over supported pairs only. Target language abbreviations: Ass=Assamese, Ben=Bengali, Guj=Gujarati, Hin=Hindi, Kan=Kannada, Mal=Malayalam, Mar=Marathi, Odi=Odia, Pun=Punjabi, Tam=Tamil, Urd=Urdu.}
\label{tab:t2_xling_tel}
\end{table*}
