# Supplementary material for: One Instruction Does Not Fit All: How Well Do Embeddings Align Personas and Instructions in Low-Resource Indian Languages?
Source: arXiv:2601.10205 source file (2026-01-15)
Supplement: Supplementary file 12 [file t2_xling_urd_to_all.tex]

\begin{table*}[t]
\centering
\tiny
\begin{tabular}{lcccccccccccc}
\toprule
\textbf{Model} & \textbf{Ass} & \textbf{Ben} & \textbf{Guj} & \textbf{Hin} & \textbf{Kan} & \textbf{Mal} & \textbf{Mar} & \textbf{Odi} & \textbf{Pun} & \textbf{Tam} & \textbf{Tel} & \textbf{Avg} \\
\midrule
\multicolumn{13}{l}{\textit{Recall@1 (\%)}} \\
multilingual-e5-large-instruct & 19.2 & 23.2 & 23.2 & 27.2 & 22.5 & 18.1 & 24.1 & 20.1 & 21.3 & 18.4 & 20.1 & 21.6 \\
LaBSE & 7.3 & 13.3 & 15.3 & 15.9 & 13.9 & 10.9 & 13.8 & 12.8 & 14.3 & 13.1 & 13.8 & 13.1 \\
Para-MPNet & -- & -- & 11.0 & 14.7 & -- & -- & 12.4 & -- & -- & -- & -- & 12.7 \\
indic-sentence-bert-nli & 10.6 & 12.9 & 12.8 & 14.5 & 12.8 & 10.9 & 11.8 & 9.9 & 14.0 & 12.1 & 12.3 & 12.2 \\
BGE-M3 & 10.0 & 12.1 & 12.9 & 14.7 & 13.1 & 11.8 & 12.5 & 10.8 & 12.8 & 10.9 & 12.7 & 12.2 \\
indic-sentence-similarity-sbert & 9.1 & 11.2 & 10.8 & 11.6 & 11.3 & 9.4 & 10.3 & 7.7 & 11.1 & 10.5 & 10.5 & 10.3 \\
Para-XLM-R & -- & -- & 7.5 & 9.5 & -- & -- & 8.5 & -- & -- & -- & -- & 8.5 \\
DistilUSE-Multi & -- & -- & 5.1 & 10.2 & -- & -- & 6.7 & -- & -- & -- & -- & 7.3 \\
\midrule
\multicolumn{13}{l}{\textit{MRR@10}} \\
multilingual-e5-large-instruct & 0.252 & 0.299 & 0.297 & 0.343 & 0.288 & 0.238 & 0.307 & 0.261 & 0.277 & 0.244 & 0.261 & 0.279 \\
LaBSE & 0.100 & 0.175 & 0.199 & 0.205 & 0.182 & 0.146 & 0.180 & 0.169 & 0.186 & 0.173 & 0.181 & 0.172 \\
Para-MPNet & -- & -- & 0.157 & 0.202 & -- & -- & 0.172 & -- & -- & -- & -- & 0.177 \\
indic-sentence-bert-nli & 0.153 & 0.178 & 0.179 & 0.199 & 0.177 & 0.155 & 0.168 & 0.143 & 0.193 & 0.169 & 0.172 & 0.171 \\
BGE-M3 & 0.137 & 0.162 & 0.172 & 0.192 & 0.172 & 0.160 & 0.167 & 0.147 & 0.171 & 0.149 & 0.170 & 0.164 \\
indic-sentence-similarity-sbert & 0.130 & 0.154 & 0.149 & 0.160 & 0.156 & 0.133 & 0.145 & 0.112 & 0.154 & 0.147 & 0.146 & 0.144 \\
Para-XLM-R & -- & -- & 0.109 & 0.138 & -- & -- & 0.124 & -- & -- & -- & -- & 0.124 \\
DistilUSE-Multi & -- & -- & 0.075 & 0.142 & -- & -- & 0.096 & -- & -- & -- & -- & 0.104 \\
\bottomrule
\end{tabular}
\caption{Cross-lingual persona$\rightarrow$instruction retrieval (T2) from Urdu to all target languages. Recall@1 (\%) and MRR@10 metrics shown for each source-target pair; averages computed over supported pairs only. Target language abbreviations: Ass=Assamese, Ben=Bengali, Guj=Gujarati, Hin=Hindi, Kan=Kannada, Mal=Malayalam, Mar=Marathi, Odi=Odia, Pun=Punjabi, Tam=Tamil, Tel=Telugu.}
\label{tab:t2_xling_urd}
\end{table*}
