# Supplementary material for: One Instruction Does Not Fit All: How Well Do Embeddings Align Personas and Instructions in Low-Resource Indian Languages?
Source: arXiv:2601.10205 source file (2026-01-15)
Supplement: Supplementary file 13 [file t3_xling_reverse_asm_to_all.tex]

\begin{table*}[t]
\centering
\tiny
\begin{tabular}{lcccccccccccc}
\toprule
\textbf{Model} & \textbf{Ben} & \textbf{Guj} & \textbf{Hin} & \textbf{Kan} & \textbf{Mal} & \textbf{Mar} & \textbf{Odi} & \textbf{Pun} & \textbf{Tam} & \textbf{Tel} & \textbf{Urd} & \textbf{Avg} \\
\midrule
\multicolumn{13}{l}{\textit{Recall@1 (\%)}} \\
multilingual-e5-large-instruct & 25.9 & 22.8 & 25.7 & 24.3 & 22.5 & 25.5 & 23.0 & 23.4 & 22.5 & 24.1 & 24.5 & 24.0 \\
BGE-M3 & 24.7 & 20.3 & 21.9 & 21.1 & 19.9 & 21.1 & 20.4 & 19.1 & 18.1 & 20.9 & 19.2 & 20.6 \\
indic-sentence-bert-nli & 17.8 & 15.3 & 16.9 & 15.8 & 13.8 & 14.9 & 12.3 & 15.9 & 14.4 & 15.5 & 14.5 & 15.2 \\
LaBSE & 14.4 & 14.2 & 15.0 & 13.8 & 11.6 & 13.4 & 13.3 & 13.3 & 13.1 & 13.6 & 13.5 & 13.6 \\
indic-sentence-similarity-sbert & 13.9 & 12.0 & 13.3 & 12.5 & 10.6 & 12.3 & 9.2 & 12.6 & 11.7 & 11.4 & 12.0 & 12.0 \\
\midrule
\multicolumn{13}{l}{\textit{MRR@10}} \\
multilingual-e5-large-instruct & 0.321 & 0.289 & 0.322 & 0.307 & 0.285 & 0.320 & 0.288 & 0.298 & 0.286 & 0.303 & 0.311 & 0.303 \\
BGE-M3 & 0.305 & 0.258 & 0.276 & 0.268 & 0.253 & 0.268 & 0.259 & 0.245 & 0.231 & 0.264 & 0.248 & 0.261 \\
indic-sentence-bert-nli & 0.236 & 0.211 & 0.228 & 0.216 & 0.192 & 0.206 & 0.172 & 0.218 & 0.200 & 0.211 & 0.200 & 0.208 \\
LaBSE & 0.190 & 0.188 & 0.198 & 0.183 & 0.157 & 0.180 & 0.176 & 0.177 & 0.177 & 0.181 & 0.181 & 0.181 \\
indic-sentence-similarity-sbert & 0.187 & 0.166 & 0.181 & 0.172 & 0.147 & 0.168 & 0.130 & 0.172 & 0.161 & 0.159 & 0.166 & 0.165 \\
\bottomrule
\end{tabular}
\caption{Cross-lingual instruction$\rightarrow$persona retrieval (T3 reverse) from Assamese to all target languages. Recall@1 (\%) and MRR@10 metrics shown for each source-target pair; averages computed over supported pairs only. Target language abbreviations: Ben=Bengali, Guj=Gujarati, Hin=Hindi, Kan=Kannada, Mal=Malayalam, Mar=Marathi, Odi=Odia, Pun=Punjabi, Tam=Tamil, Tel=Telugu, Urd=Urdu.}
\label{tab:t3_xling_reverse_asm}
\end{table*}
