# Supplementary material for: One Instruction Does Not Fit All: How Well Do Embeddings Align Personas and Instructions in Low-Resource Indian Languages?
Source: arXiv:2601.10205 source file (2026-01-15)
Supplement: Supplementary file 14 [file t3_xling_reverse_ben_to_all.tex]

\begin{table*}[t]
\centering
\tiny
\begin{tabular}{lcccccccccccc}
\toprule
\textbf{Model} & \textbf{Ass} & \textbf{Guj} & \textbf{Hin} & \textbf{Kan} & \textbf{Mal} & \textbf{Mar} & \textbf{Odi} & \textbf{Pun} & \textbf{Tam} & \textbf{Tel} & \textbf{Urd} & \textbf{Avg} \\
\midrule
\multicolumn{13}{l}{\textit{Recall@1 (\%)}} \\
multilingual-e5-large-instruct & 27.0 & 27.9 & 31.5 & 29.5 & 27.4 & 31.2 & 27.3 & 28.6 & 27.4 & 28.9 & 30.3 & 28.8 \\
BGE-M3 & 25.3 & 25.0 & 27.3 & 26.4 & 24.5 & 26.2 & 24.2 & 23.4 & 22.3 & 25.9 & 24.1 & 25.0 \\
indic-sentence-bert-nli & 15.8 & 17.6 & 20.0 & 18.4 & 15.7 & 16.6 & 12.7 & 18.3 & 16.6 & 17.3 & 16.1 & 16.8 \\
LaBSE & 9.0 & 18.5 & 19.9 & 17.6 & 13.6 & 16.8 & 15.9 & 16.5 & 16.7 & 17.0 & 17.5 & 16.3 \\
indic-sentence-similarity-sbert & 14.9 & 15.3 & 17.1 & 16.0 & 12.9 & 15.2 & 10.2 & 15.7 & 14.5 & 14.4 & 14.7 & 14.6 \\
\midrule
\multicolumn{13}{l}{\textit{MRR@10}} \\
multilingual-e5-large-instruct & 0.332 & 0.346 & 0.386 & 0.366 & 0.341 & 0.383 & 0.337 & 0.356 & 0.342 & 0.357 & 0.375 & 0.356 \\
BGE-M3 & 0.313 & 0.311 & 0.336 & 0.325 & 0.306 & 0.325 & 0.302 & 0.291 & 0.279 & 0.320 & 0.302 & 0.310 \\
indic-sentence-bert-nli & 0.213 & 0.238 & 0.264 & 0.246 & 0.214 & 0.228 & 0.178 & 0.244 & 0.227 & 0.234 & 0.220 & 0.228 \\
LaBSE & 0.123 & 0.238 & 0.254 & 0.227 & 0.178 & 0.219 & 0.205 & 0.213 & 0.216 & 0.219 & 0.226 & 0.211 \\
indic-sentence-similarity-sbert & 0.201 & 0.204 & 0.226 & 0.213 & 0.176 & 0.203 & 0.144 & 0.211 & 0.197 & 0.196 & 0.201 & 0.197 \\
\bottomrule
\end{tabular}
\caption{Cross-lingual instruction$\rightarrow$persona retrieval (T3 reverse) from Bengali to all target languages. Recall@1 (\%) and MRR@10 metrics shown for each source-target pair; averages computed over supported pairs only. Target language abbreviations: Ass=Assamese, Guj=Gujarati, Hin=Hindi, Kan=Kannada, Mal=Malayalam, Mar=Marathi, Odi=Odia, Pun=Punjabi, Tam=Tamil, Tel=Telugu, Urd=Urdu.}
\label{tab:t3_xling_reverse_ben}
\end{table*}
