# Supplementary material for: One Instruction Does Not Fit All: How Well Do Embeddings Align Personas and Instructions in Low-Resource Indian Languages?
Source: arXiv:2601.10205 source file (2026-01-15)
Supplement: Supplementary file 15 [file t3_xling_reverse_guj_to_all.tex]

\begin{table*}[t]
\centering
\tiny
\begin{tabular}{lcccccccccccc}
\toprule
\textbf{Model} & \textbf{Ass} & \textbf{Ben} & \textbf{Hin} & \textbf{Kan} & \textbf{Mal} & \textbf{Mar} & \textbf{Odi} & \textbf{Pun} & \textbf{Tam} & \textbf{Tel} & \textbf{Urd} & \textbf{Avg} \\
\midrule
\multicolumn{13}{l}{\textit{Recall@1 (\%)}} \\
multilingual-e5-large-instruct & 23.9 & 26.6 & 27.1 & 27.6 & 24.1 & 28.1 & 24.6 & 28.2 & 23.4 & 25.0 & 26.2 & 25.9 \\
BGE-M3 & 20.3 & 24.5 & 27.3 & 25.9 & 24.0 & 26.5 & 22.9 & 24.2 & 21.0 & 25.1 & 23.5 & 24.1 \\
indic-sentence-bert-nli & 14.2 & 17.5 & 19.2 & 18.1 & 15.5 & 16.9 & 12.7 & 18.4 & 16.0 & 17.5 & 13.3 & 16.3 \\
LaBSE & 6.8 & 16.1 & 20.5 & 17.4 & 12.5 & 16.7 & 14.7 & 16.6 & 16.3 & 16.8 & 17.7 & 15.6 \\
Para-MPNet & -- & -- & 16.1 & -- & -- & 14.1 & -- & -- & -- & -- & 13.5 & 14.6 \\
Para-XLM-R & -- & -- & 15.9 & -- & -- & 13.2 & -- & -- & -- & -- & 12.8 & 14.0 \\
indic-sentence-similarity-sbert & 12.7 & 14.6 & 15.9 & 14.9 & 12.1 & 14.5 & 9.7 & 15.3 & 13.2 & 13.9 & 14.2 & 13.7 \\
DistilUSE-Multi & -- & -- & 8.0 & -- & -- & 6.3 & -- & -- & -- & -- & 6.9 & 7.1 \\
\midrule
\multicolumn{13}{l}{\textit{MRR@10}} \\
multilingual-e5-large-instruct & 0.300 & 0.329 & 0.337 & 0.339 & 0.304 & 0.347 & 0.304 & 0.348 & 0.296 & 0.312 & 0.326 & 0.322 \\
BGE-M3 & 0.258 & 0.304 & 0.335 & 0.320 & 0.298 & 0.326 & 0.286 & 0.301 & 0.264 & 0.308 & 0.294 & 0.299 \\
indic-sentence-bert-nli & 0.198 & 0.238 & 0.257 & 0.243 & 0.211 & 0.229 & 0.178 & 0.245 & 0.220 & 0.236 & 0.195 & 0.223 \\
LaBSE & 0.095 & 0.209 & 0.259 & 0.222 & 0.166 & 0.216 & 0.191 & 0.213 & 0.211 & 0.214 & 0.227 & 0.202 \\
Para-MPNet & -- & -- & 0.219 & -- & -- & 0.194 & -- & -- & -- & -- & 0.188 & 0.200 \\
Para-XLM-R & -- & -- & 0.216 & -- & -- & 0.181 & -- & -- & -- & -- & 0.178 & 0.192 \\
indic-sentence-similarity-sbert & 0.173 & 0.197 & 0.212 & 0.200 & 0.166 & 0.194 & 0.136 & 0.205 & 0.181 & 0.187 & 0.193 & 0.186 \\
DistilUSE-Multi & -- & -- & 0.114 & -- & -- & 0.091 & -- & -- & -- & -- & 0.100 & 0.102 \\
\bottomrule
\end{tabular}
\caption{Cross-lingual instruction$\rightarrow$persona retrieval (T3 reverse) from Gujarati to all target languages. Recall@1 (\%) and MRR@10 metrics shown for each source-target pair; averages computed over supported pairs only. Target language abbreviations: Ass=Assamese, Ben=Bengali, Hin=Hindi, Kan=Kannada, Mal=Malayalam, Mar=Marathi, Odi=Odia, Pun=Punjabi, Tam=Tamil, Tel=Telugu, Urd=Urdu.}
\label{tab:t3_xling_reverse_guj}
\end{table*}
