# Supplementary material for: One Instruction Does Not Fit All: How Well Do Embeddings Align Personas and Instructions in Low-Resource Indian Languages?
Source: arXiv:2601.10205 source file (2026-01-15)
Supplement: Supplementary file 16 [file t3_xling_reverse_hin_to_all.tex]

\begin{table*}[t]
\centering
\tiny
\begin{tabular}{lcccccccccccc}
\toprule
\textbf{Model} & \textbf{Ass} & \textbf{Ben} & \textbf{Guj} & \textbf{Kan} & \textbf{Mal} & \textbf{Mar} & \textbf{Odi} & \textbf{Pun} & \textbf{Tam} & \textbf{Tel} & \textbf{Urd} & \textbf{Avg} \\
\midrule
\multicolumn{13}{l}{\textit{Recall@1 (\%)}} \\
multilingual-e5-large-instruct & 28.5 & 33.2 & 31.4 & 32.7 & 30.1 & 33.9 & 30.1 & 32.2 & 30.4 & 31.9 & 33.7 & 31.6 \\
BGE-M3 & 21.7 & 26.2 & 27.1 & 27.4 & 25.2 & 31.1 & 24.1 & 25.5 & 22.6 & 26.4 & 25.9 & 25.7 \\
Para-MPNet & -- & -- & 16.8 & -- & -- & 21.3 & -- & -- & -- & -- & 18.1 & 18.7 \\
indic-sentence-bert-nli & 16.3 & 19.9 & 19.5 & 20.2 & 16.8 & 20.8 & 14.1 & 20.5 & 18.2 & 18.9 & 8.5 & 17.6 \\
Para-XLM-R & -- & -- & 15.7 & -- & -- & 18.4 & -- & -- & -- & -- & 16.7 & 16.9 \\
LaBSE & 6.6 & 16.1 & 19.3 & 17.5 & 12.4 & 17.7 & 14.8 & 16.6 & 16.7 & 16.8 & 17.9 & 15.7 \\
indic-sentence-similarity-sbert & 13.8 & 16.6 & 16.1 & 16.7 & 13.3 & 17.7 & 10.2 & 17.0 & 15.0 & 14.8 & 15.5 & 15.2 \\
DistilUSE-Multi & -- & -- & 8.8 & -- & -- & 14.6 & -- & -- & -- & -- & 14.1 & 12.5 \\
\midrule
\multicolumn{13}{l}{\textit{MRR@10}} \\
multilingual-e5-large-instruct & 0.354 & 0.405 & 0.386 & 0.399 & 0.372 & 0.411 & 0.370 & 0.396 & 0.376 & 0.390 & 0.413 & 0.388 \\
BGE-M3 & 0.275 & 0.325 & 0.332 & 0.337 & 0.314 & 0.378 & 0.301 & 0.316 & 0.284 & 0.326 & 0.322 & 0.319 \\
Para-MPNet & -- & -- & 0.226 & -- & -- & 0.277 & -- & -- & -- & -- & 0.242 & 0.248 \\
indic-sentence-bert-nli & 0.222 & 0.265 & 0.260 & 0.268 & 0.227 & 0.275 & 0.196 & 0.271 & 0.246 & 0.253 & 0.121 & 0.237 \\
Para-XLM-R & -- & -- & 0.213 & -- & -- & 0.244 & -- & -- & -- & -- & 0.226 & 0.228 \\
LaBSE & 0.093 & 0.209 & 0.244 & 0.224 & 0.164 & 0.227 & 0.192 & 0.214 & 0.215 & 0.215 & 0.230 & 0.202 \\
indic-sentence-similarity-sbert & 0.188 & 0.222 & 0.215 & 0.221 & 0.182 & 0.232 & 0.144 & 0.225 & 0.203 & 0.201 & 0.209 & 0.204 \\
DistilUSE-Multi & -- & -- & 0.122 & -- & -- & 0.195 & -- & -- & -- & -- & 0.190 & 0.169 \\
\bottomrule
\end{tabular}
\caption{Cross-lingual instruction$\rightarrow$persona retrieval (T3 reverse) from Hindi to all target languages. Recall@1 (\%) and MRR@10 metrics shown for each source-target pair; averages computed over supported pairs only. Target language abbreviations: Ass=Assamese, Ben=Bengali, Guj=Gujarati, Kan=Kannada, Mal=Malayalam, Mar=Marathi, Odi=Odia, Pun=Punjabi, Tam=Tamil, Tel=Telugu, Urd=Urdu.}
\label{tab:t3_xling_reverse_hin}
\end{table*}
