# Supplementary material for: One Instruction Does Not Fit All: How Well Do Embeddings Align Personas and Instructions in Low-Resource Indian Languages?
Source: arXiv:2601.10205 source file (2026-01-15)
Supplement: Supplementary file 17 [file t3_xling_reverse_kan_to_all.tex]

\begin{table*}[t]
\centering
\tiny
\begin{tabular}{lcccccccccccc}
\toprule
\textbf{Model} & \textbf{Ass} & \textbf{Ben} & \textbf{Guj} & \textbf{Hin} & \textbf{Mal} & \textbf{Mar} & \textbf{Odi} & \textbf{Pun} & \textbf{Tam} & \textbf{Tel} & \textbf{Urd} & \textbf{Avg} \\
\midrule
\multicolumn{13}{l}{\textit{Recall@1 (\%)}} \\
multilingual-e5-large-instruct & 24.4 & 28.3 & 26.8 & 30.9 & 27.1 & 30.1 & 25.9 & 27.9 & 26.7 & 29.0 & 27.9 & 27.7 \\
BGE-M3 & 20.3 & 24.4 & 24.8 & 26.6 & 25.2 & 25.9 & 22.8 & 22.8 & 22.6 & 26.7 & 23.2 & 24.1 \\
indic-sentence-bert-nli & 15.6 & 18.4 & 17.9 & 20.4 & 17.0 & 17.5 & 13.2 & 18.9 & 17.3 & 18.8 & 16.7 & 17.4 \\
LaBSE & 8.0 & 16.7 & 19.2 & 20.4 & 14.1 & 17.5 & 15.6 & 16.8 & 17.6 & 18.1 & 18.0 & 16.6 \\
indic-sentence-similarity-sbert & 13.5 & 15.8 & 15.2 & 16.8 & 13.5 & 15.2 & 10.1 & 15.7 & 15.2 & 15.4 & 14.7 & 14.7 \\
\midrule
\multicolumn{13}{l}{\textit{MRR@10}} \\
multilingual-e5-large-instruct & 0.309 & 0.353 & 0.336 & 0.381 & 0.337 & 0.371 & 0.324 & 0.347 & 0.333 & 0.356 & 0.349 & 0.345 \\
BGE-M3 & 0.259 & 0.305 & 0.307 & 0.329 & 0.312 & 0.321 & 0.286 & 0.285 & 0.284 & 0.326 & 0.292 & 0.301 \\
indic-sentence-bert-nli & 0.213 & 0.248 & 0.242 & 0.269 & 0.229 & 0.237 & 0.185 & 0.251 & 0.236 & 0.250 & 0.225 & 0.235 \\
LaBSE & 0.111 & 0.217 & 0.244 & 0.259 & 0.183 & 0.226 & 0.201 & 0.217 & 0.226 & 0.230 & 0.231 & 0.213 \\
indic-sentence-similarity-sbert & 0.183 & 0.211 & 0.203 & 0.223 & 0.183 & 0.204 & 0.142 & 0.210 & 0.205 & 0.205 & 0.199 & 0.197 \\
\bottomrule
\end{tabular}
\caption{Cross-lingual instruction$\rightarrow$persona retrieval (T3 reverse) from Kannada to all target languages. Recall@1 (\%) and MRR@10 metrics shown for each source-target pair; averages computed over supported pairs only. Target language abbreviations: Ass=Assamese, Ben=Bengali, Guj=Gujarati, Hin=Hindi, Mal=Malayalam, Mar=Marathi, Odi=Odia, Pun=Punjabi, Tam=Tamil, Tel=Telugu, Urd=Urdu.}
\label{tab:t3_xling_reverse_kan}
\end{table*}
