# Supplementary material for: One Instruction Does Not Fit All: How Well Do Embeddings Align Personas and Instructions in Low-Resource Indian Languages?
Source: arXiv:2601.10205 source file (2026-01-15)
Supplement: Supplementary file 18 [file t3_xling_reverse_mal_to_all.tex]

\begin{table*}[t]
\centering
\tiny
\begin{tabular}{lcccccccccccc}
\toprule
\textbf{Model} & \textbf{Ass} & \textbf{Ben} & \textbf{Guj} & \textbf{Hin} & \textbf{Kan} & \textbf{Mar} & \textbf{Odi} & \textbf{Pun} & \textbf{Tam} & \textbf{Tel} & \textbf{Urd} & \textbf{Avg} \\
\midrule
\multicolumn{13}{l}{\textit{Recall@1 (\%)}} \\
multilingual-e5-large-instruct & 24.2 & 27.6 & 27.0 & 29.3 & 27.2 & 29.5 & 22.9 & 26.4 & 25.7 & 27.9 & 28.1 & 26.9 \\
BGE-M3 & 20.0 & 24.3 & 24.2 & 25.8 & 26.3 & 25.0 & 22.2 & 22.4 & 22.9 & 26.0 & 23.6 & 23.9 \\
LaBSE & 9.0 & 16.2 & 18.2 & 18.8 & 17.9 & 16.9 & 15.3 & 16.5 & 17.4 & 17.6 & 17.2 & 16.5 \\
indic-sentence-bert-nli & 12.7 & 15.7 & 15.1 & 16.8 & 16.2 & 14.3 & 11.4 & 16.1 & 15.1 & 15.7 & 13.7 & 14.8 \\
indic-sentence-similarity-sbert & 11.4 & 13.2 & 12.8 & 13.9 & 13.7 & 12.6 & 8.8 & 13.4 & 12.9 & 13.0 & 12.6 & 12.6 \\
\midrule
\multicolumn{13}{l}{\textit{MRR@10}} \\
multilingual-e5-large-instruct & 0.305 & 0.344 & 0.336 & 0.365 & 0.337 & 0.365 & 0.289 & 0.331 & 0.324 & 0.344 & 0.350 & 0.335 \\
BGE-M3 & 0.256 & 0.304 & 0.301 & 0.321 & 0.325 & 0.313 & 0.280 & 0.282 & 0.287 & 0.321 & 0.297 & 0.299 \\
LaBSE & 0.124 & 0.212 & 0.233 & 0.242 & 0.230 & 0.220 & 0.200 & 0.214 & 0.223 & 0.226 & 0.223 & 0.213 \\
indic-sentence-bert-nli & 0.179 & 0.215 & 0.208 & 0.228 & 0.220 & 0.200 & 0.162 & 0.220 & 0.208 & 0.216 & 0.192 & 0.204 \\
indic-sentence-similarity-sbert & 0.158 & 0.180 & 0.175 & 0.188 & 0.186 & 0.172 & 0.125 & 0.183 & 0.176 & 0.177 & 0.173 & 0.172 \\
\bottomrule
\end{tabular}
\caption{Cross-lingual instruction$\rightarrow$persona retrieval (T3 reverse) from Malayalam to all target languages. Recall@1 (\%) and MRR@10 metrics shown for each source-target pair; averages computed over supported pairs only. Target language abbreviations: Ass=Assamese, Ben=Bengali, Guj=Gujarati, Hin=Hindi, Kan=Kannada, Mar=Marathi, Odi=Odia, Pun=Punjabi, Tam=Tamil, Tel=Telugu, Urd=Urdu.}
\label{tab:t3_xling_reverse_mal}
\end{table*}
