# Supplementary material for: One Instruction Does Not Fit All: How Well Do Embeddings Align Personas and Instructions in Low-Resource Indian Languages?
Source: arXiv:2601.10205 source file (2026-01-15)
Supplement: Supplementary file 19 [file t3_xling_reverse_mar_to_all.tex]

\begin{table*}[t]
\centering
\tiny
\begin{tabular}{lcccccccccccc}
\toprule
\textbf{Model} & \textbf{Ass} & \textbf{Ben} & \textbf{Guj} & \textbf{Hin} & \textbf{Kan} & \textbf{Mal} & \textbf{Odi} & \textbf{Pun} & \textbf{Tam} & \textbf{Tel} & \textbf{Urd} & \textbf{Avg} \\
\midrule
\multicolumn{13}{l}{\textit{Recall@1 (\%)}} \\
multilingual-e5-large-instruct & 26.3 & 30.3 & 29.0 & 34.1 & 29.4 & 27.4 & 27.1 & 29.2 & 27.2 & 28.7 & 29.9 & 29.0 \\
BGE-M3 & 21.1 & 25.1 & 25.9 & 30.9 & 26.4 & 24.5 & 22.9 & 23.7 & 22.1 & 25.7 & 24.1 & 24.8 \\
LaBSE & 8.3 & 17.3 & 19.7 & 22.1 & 18.5 & 14.0 & 16.1 & 17.3 & 17.5 & 18.0 & 18.3 & 17.0 \\
Para-MPNet & -- & -- & 14.5 & 20.8 & -- & -- & -- & -- & -- & -- & 15.4 & 16.9 \\
Para-XLM-R & -- & -- & 13.2 & 19.1 & -- & -- & -- & -- & -- & -- & 13.7 & 15.3 \\
indic-sentence-similarity-sbert & 12.4 & 14.7 & 14.4 & 17.5 & 14.9 & 11.9 & 9.2 & 14.9 & 13.4 & 13.6 & 13.6 & 13.7 \\
indic-sentence-bert-nli & 9.7 & 16.4 & 13.7 & 13.8 & 16.2 & 13.3 & 4.5 & 16.4 & 14.6 & 15.7 & 12.0 & 13.3 \\
DistilUSE-Multi & -- & -- & 6.5 & 13.1 & -- & -- & -- & -- & -- & -- & 9.5 & 9.7 \\
\midrule
\multicolumn{13}{l}{\textit{MRR@10}} \\
multilingual-e5-large-instruct & 0.329 & 0.373 & 0.360 & 0.414 & 0.363 & 0.343 & 0.337 & 0.363 & 0.341 & 0.355 & 0.370 & 0.359 \\
BGE-M3 & 0.266 & 0.312 & 0.320 & 0.373 & 0.327 & 0.305 & 0.288 & 0.296 & 0.277 & 0.318 & 0.303 & 0.308 \\
LaBSE & 0.114 & 0.224 & 0.249 & 0.277 & 0.236 & 0.183 & 0.208 & 0.222 & 0.225 & 0.230 & 0.235 & 0.218 \\
Para-MPNet & -- & -- & 0.198 & 0.273 & -- & -- & -- & -- & -- & -- & 0.210 & 0.227 \\
Para-XLM-R & -- & -- & 0.182 & 0.253 & -- & -- & -- & -- & -- & -- & 0.192 & 0.209 \\
indic-sentence-similarity-sbert & 0.171 & 0.198 & 0.193 & 0.229 & 0.199 & 0.165 & 0.132 & 0.200 & 0.183 & 0.184 & 0.186 & 0.186 \\
indic-sentence-bert-nli & 0.155 & 0.226 & 0.199 & 0.201 & 0.224 & 0.188 & 0.118 & 0.226 & 0.205 & 0.217 & 0.171 & 0.194 \\
DistilUSE-Multi & -- & -- & 0.093 & 0.178 & -- & -- & -- & -- & -- & -- & 0.135 & 0.135 \\
\bottomrule
\end{tabular}
\caption{Cross-lingual instruction$\rightarrow$persona retrieval (T3 reverse) from Marathi to all target languages. Recall@1 (\%) and MRR@10 metrics shown for each source-target pair; averages computed over supported pairs only. Target language abbreviations: Ass=Assamese, Ben=Bengali, Guj=Gujarati, Hin=Hindi, Kan=Kannada, Mal=Malayalam, Odi=Odia, Pun=Punjabi, Tam=Tamil, Tel=Telugu, Urd=Urdu.}
\label{tab:t3_xling_reverse_mar}
\end{table*}
