# Supplementary material for: One Instruction Does Not Fit All: How Well Do Embeddings Align Personas and Instructions in Low-Resource Indian Languages?
Source: arXiv:2601.10205 source file (2026-01-15)
Supplement: Supplementary file 20 [file t3_xling_reverse_ory_to_all.tex]

\begin{table*}[t]
\centering
\tiny
\begin{tabular}{lcccccccccccc}
\toprule
\textbf{Model} & \textbf{Ass} & \textbf{Ben} & \textbf{Guj} & \textbf{Hin} & \textbf{Kan} & \textbf{Mal} & \textbf{Mar} & \textbf{Pun} & \textbf{Tam} & \textbf{Tel} & \textbf{Urd} & \textbf{Avg} \\
\midrule
\multicolumn{13}{l}{\textit{Recall@1 (\%)}} \\
multilingual-e5-large-instruct & 23.2 & 26.0 & 24.4 & 26.7 & 25.0 & 23.1 & 26.3 & 26.0 & 21.9 & 24.4 & 24.7 & 24.7 \\
BGE-M3 & 20.5 & 23.8 & 22.8 & 24.5 & 23.8 & 22.1 & 23.5 & 21.7 & 19.8 & 23.1 & 21.0 & 22.4 \\
LaBSE & 8.1 & 16.0 & 17.6 & 18.5 & 16.6 & 12.7 & 15.8 & 15.8 & 15.7 & 15.9 & 16.4 & 15.4 \\
indic-sentence-bert-nli & 6.5 & 15.3 & 14.5 & 16.1 & 15.6 & 13.3 & 13.9 & 15.4 & 13.8 & 15.3 & 13.6 & 13.9 \\
indic-sentence-similarity-sbert & 10.1 & 10.9 & 10.7 & 11.6 & 11.0 & 9.3 & 10.4 & 11.2 & 10.1 & 10.2 & 10.4 & 10.5 \\
\midrule
\multicolumn{13}{l}{\textit{MRR@10}} \\
multilingual-e5-large-instruct & 0.291 & 0.323 & 0.305 & 0.332 & 0.312 & 0.291 & 0.328 & 0.324 & 0.280 & 0.305 & 0.311 & 0.309 \\
BGE-M3 & 0.259 & 0.296 & 0.286 & 0.304 & 0.297 & 0.278 & 0.295 & 0.273 & 0.251 & 0.287 & 0.268 & 0.281 \\
LaBSE & 0.111 & 0.208 & 0.225 & 0.238 & 0.214 & 0.168 & 0.207 & 0.204 & 0.205 & 0.205 & 0.213 & 0.200 \\
indic-sentence-bert-nli & 0.104 & 0.209 & 0.199 & 0.219 & 0.213 & 0.184 & 0.193 & 0.211 & 0.192 & 0.206 & 0.189 & 0.193 \\
indic-sentence-similarity-sbert & 0.139 & 0.151 & 0.149 & 0.159 & 0.152 & 0.132 & 0.145 & 0.155 & 0.141 & 0.143 & 0.146 & 0.146 \\
\bottomrule
\end{tabular}
\caption{Cross-lingual instruction$\rightarrow$persona retrieval (T3 reverse) from Odia to all target languages. Recall@1 (\%) and MRR@10 metrics shown for each source-target pair; averages computed over supported pairs only. Target language abbreviations: Ass=Assamese, Ben=Bengali, Guj=Gujarati, Hin=Hindi, Kan=Kannada, Mal=Malayalam, Mar=Marathi, Pun=Punjabi, Tam=Tamil, Tel=Telugu, Urd=Urdu.}
\label{tab:t3_xling_reverse_ory}
\end{table*}
