# Supplementary material for: One Instruction Does Not Fit All: How Well Do Embeddings Align Personas and Instructions in Low-Resource Indian Languages?
Source: arXiv:2601.10205 source file (2026-01-15)
Supplement: Supplementary file 21 [file t3_xling_reverse_pan_to_all.tex]

\begin{table*}[t]
\centering
\tiny
\begin{tabular}{lcccccccccccc}
\toprule
\textbf{Model} & \textbf{Ass} & \textbf{Ben} & \textbf{Guj} & \textbf{Hin} & \textbf{Kan} & \textbf{Mal} & \textbf{Mar} & \textbf{Odi} & \textbf{Tam} & \textbf{Tel} & \textbf{Urd} & \textbf{Avg} \\
\midrule
\multicolumn{13}{l}{\textit{Recall@1 (\%)}} \\
multilingual-e5-large-instruct & 20.8 & 23.8 & 23.7 & 25.1 & 23.5 & 22.1 & 25.2 & 20.4 & 21.6 & 22.5 & 23.2 & 22.9 \\
BGE-M3 & 19.3 & 23.0 & 24.4 & 25.9 & 24.1 & 22.4 & 24.2 & 21.8 & 20.0 & 23.4 & 23.0 & 22.9 \\
indic-sentence-bert-nli & 13.4 & 17.4 & 17.5 & 19.9 & 18.1 & 15.4 & 16.8 & 12.8 & 16.1 & 17.3 & 11.7 & 16.0 \\
LaBSE & 7.2 & 15.1 & 17.7 & 19.0 & 16.6 & 12.5 & 15.6 & 14.1 & 15.4 & 15.8 & 17.0 & 15.1 \\
indic-sentence-similarity-sbert & 12.7 & 14.9 & 15.0 & 16.4 & 15.1 & 12.4 & 14.3 & 10.0 & 13.6 & 13.7 & 14.6 & 13.9 \\
\midrule
\multicolumn{13}{l}{\textit{MRR@10}} \\
multilingual-e5-large-instruct & 0.263 & 0.297 & 0.294 & 0.314 & 0.293 & 0.278 & 0.313 & 0.256 & 0.273 & 0.283 & 0.292 & 0.287 \\
BGE-M3 & 0.246 & 0.287 & 0.302 & 0.318 & 0.299 & 0.282 & 0.301 & 0.274 & 0.252 & 0.291 & 0.289 & 0.286 \\
indic-sentence-bert-nli & 0.189 & 0.236 & 0.236 & 0.262 & 0.243 & 0.211 & 0.230 & 0.179 & 0.221 & 0.234 & 0.162 & 0.219 \\
LaBSE & 0.099 & 0.198 & 0.226 & 0.242 & 0.212 & 0.165 & 0.203 & 0.183 & 0.200 & 0.203 & 0.217 & 0.195 \\
indic-sentence-similarity-sbert & 0.175 & 0.200 & 0.201 & 0.217 & 0.201 & 0.170 & 0.194 & 0.140 & 0.185 & 0.187 & 0.197 & 0.188 \\
\bottomrule
\end{tabular}
\caption{Cross-lingual instruction$\rightarrow$persona retrieval (T3 reverse) from Punjabi to all target languages. Recall@1 (\%) and MRR@10 metrics shown for each source-target pair; averages computed over supported pairs only. Target language abbreviations: Ass=Assamese, Ben=Bengali, Guj=Gujarati, Hin=Hindi, Kan=Kannada, Mal=Malayalam, Mar=Marathi, Odi=Odia, Tam=Tamil, Tel=Telugu, Urd=Urdu.}
\label{tab:t3_xling_reverse_pan}
\end{table*}
