# Supplementary material for: One Instruction Does Not Fit All: How Well Do Embeddings Align Personas and Instructions in Low-Resource Indian Languages?
Source: arXiv:2601.10205 source file (2026-01-15)
Supplement: Supplementary file 22 [file t3_xling_reverse_tam_to_all.tex]

\begin{table*}[t]
\centering
\tiny
\begin{tabular}{lcccccccccccc}
\toprule
\textbf{Model} & \textbf{Ass} & \textbf{Ben} & \textbf{Guj} & \textbf{Hin} & \textbf{Kan} & \textbf{Mal} & \textbf{Mar} & \textbf{Odi} & \textbf{Pun} & \textbf{Tel} & \textbf{Urd} & \textbf{Avg} \\
\midrule
\multicolumn{13}{l}{\textit{Recall@1 (\%)}} \\
multilingual-e5-large-instruct & 23.6 & 26.8 & 24.8 & 28.2 & 27.9 & 25.1 & 27.7 & 24.3 & 25.5 & 26.6 & 27.1 & 26.2 \\
BGE-M3 & 17.6 & 21.3 & 20.9 & 23.0 & 24.0 & 22.6 & 22.2 & 19.4 & 19.7 & 23.4 & 21.1 & 21.4 \\
indic-sentence-bert-nli & 14.3 & 17.0 & 16.4 & 18.5 & 17.9 & 16.0 & 16.0 & 12.0 & 17.1 & 17.4 & 15.2 & 16.2 \\
LaBSE & 7.3 & 15.5 & 17.7 & 19.1 & 17.2 & 13.3 & 16.2 & 14.3 & 15.6 & 16.6 & 16.9 & 15.4 \\
indic-sentence-similarity-sbert & 12.5 & 14.5 & 13.9 & 15.5 & 15.3 & 12.7 & 13.7 & 9.3 & 14.5 & 14.2 & 13.8 & 13.6 \\
\midrule
\multicolumn{13}{l}{\textit{MRR@10}} \\
multilingual-e5-large-instruct & 0.298 & 0.337 & 0.313 & 0.352 & 0.346 & 0.318 & 0.346 & 0.308 & 0.323 & 0.331 & 0.340 & 0.328 \\
BGE-M3 & 0.228 & 0.270 & 0.265 & 0.289 & 0.299 & 0.284 & 0.281 & 0.250 & 0.252 & 0.291 & 0.268 & 0.271 \\
indic-sentence-bert-nli & 0.198 & 0.230 & 0.224 & 0.248 & 0.241 & 0.217 & 0.220 & 0.170 & 0.231 & 0.234 & 0.208 & 0.220 \\
LaBSE & 0.102 & 0.203 & 0.227 & 0.244 & 0.221 & 0.175 & 0.209 & 0.187 & 0.203 & 0.214 & 0.218 & 0.200 \\
indic-sentence-similarity-sbert & 0.171 & 0.196 & 0.188 & 0.207 & 0.204 & 0.174 & 0.187 & 0.132 & 0.195 & 0.191 & 0.188 & 0.185 \\
\bottomrule
\end{tabular}
\caption{Cross-lingual instruction$\rightarrow$persona retrieval (T3 reverse) from Tamil to all target languages. Recall@1 (\%) and MRR@10 metrics shown for each source-target pair; averages computed over supported pairs only. Target language abbreviations: Ass=Assamese, Ben=Bengali, Guj=Gujarati, Hin=Hindi, Kan=Kannada, Mal=Malayalam, Mar=Marathi, Odi=Odia, Pun=Punjabi, Tel=Telugu, Urd=Urdu.}
\label{tab:t3_xling_reverse_tam}
\end{table*}
