# Supplementary material for: One Instruction Does Not Fit All: How Well Do Embeddings Align Personas and Instructions in Low-Resource Indian Languages?
Source: arXiv:2601.10205 source file (2026-01-15)
Supplement: Supplementary file 23 [file t3_xling_reverse_tel_to_all.tex]

\begin{table*}[t]
\centering
\tiny
\begin{tabular}{lcccccccccccc}
\toprule
\textbf{Model} & \textbf{Ass} & \textbf{Ben} & \textbf{Guj} & \textbf{Hin} & \textbf{Kan} & \textbf{Mal} & \textbf{Mar} & \textbf{Odi} & \textbf{Pun} & \textbf{Tam} & \textbf{Urd} & \textbf{Avg} \\
\midrule
\multicolumn{13}{l}{\textit{Recall@1 (\%)}} \\
multilingual-e5-large-instruct & 24.7 & 29.1 & 27.4 & 30.2 & 29.1 & 27.5 & 29.9 & 25.4 & 27.8 & 26.7 & 28.7 & 27.9 \\
BGE-M3 & 20.5 & 24.9 & 24.8 & 26.6 & 27.5 & 25.6 & 26.1 & 22.8 & 23.3 & 23.1 & 24.1 & 24.5 \\
LaBSE & 7.7 & 16.3 & 19.0 & 20.2 & 18.4 & 14.0 & 17.1 & 15.1 & 16.5 & 17.3 & 17.8 & 16.3 \\
indic-sentence-bert-nli & 11.7 & 16.6 & 16.4 & 18.1 & 17.6 & 15.3 & 15.5 & 12.4 & 17.1 & 16.0 & 13.7 & 15.5 \\
indic-sentence-similarity-sbert & 12.2 & 14.2 & 14.0 & 15.1 & 15.2 & 12.7 & 13.6 & 9.6 & 14.6 & 13.9 & 13.7 & 13.5 \\
\midrule
\multicolumn{13}{l}{\textit{MRR@10}} \\
multilingual-e5-large-instruct & 0.313 & 0.361 & 0.344 & 0.374 & 0.358 & 0.343 & 0.369 & 0.319 & 0.349 & 0.334 & 0.357 & 0.347 \\
BGE-M3 & 0.261 & 0.310 & 0.308 & 0.328 & 0.337 & 0.316 & 0.323 & 0.286 & 0.291 & 0.288 & 0.301 & 0.305 \\
LaBSE & 0.106 & 0.213 & 0.241 & 0.256 & 0.234 & 0.182 & 0.221 & 0.196 & 0.213 & 0.222 & 0.228 & 0.210 \\
indic-sentence-bert-nli & 0.169 & 0.224 & 0.223 & 0.241 & 0.235 & 0.208 & 0.213 & 0.173 & 0.230 & 0.218 & 0.192 & 0.212 \\
indic-sentence-similarity-sbert & 0.169 & 0.192 & 0.188 & 0.202 & 0.202 & 0.173 & 0.184 & 0.136 & 0.195 & 0.187 & 0.187 & 0.183 \\
\bottomrule
\end{tabular}
\caption{Cross-lingual instruction$\rightarrow$persona retrieval (T3 reverse) from Telugu to all target languages. Recall@1 (\%) and MRR@10 metrics shown for each source-target pair; averages computed over supported pairs only. Target language abbreviations: Ass=Assamese, Ben=Bengali, Guj=Gujarati, Hin=Hindi, Kan=Kannada, Mal=Malayalam, Mar=Marathi, Odi=Odia, Pun=Punjabi, Tam=Tamil, Urd=Urdu.}
\label{tab:t3_xling_reverse_tel}
\end{table*}
