# Supplementary material for: One Instruction Does Not Fit All: How Well Do Embeddings Align Personas and Instructions in Low-Resource Indian Languages?
Source: arXiv:2601.10205 source file (2026-01-15)
Supplement: Supplementary file 24 [file t3_xling_reverse_urd_to_all.tex]

\begin{table*}[t]
\centering
\tiny
\begin{tabular}{lcccccccccccc}
\toprule
\textbf{Model} & \textbf{Ass} & \textbf{Ben} & \textbf{Guj} & \textbf{Hin} & \textbf{Kan} & \textbf{Mal} & \textbf{Mar} & \textbf{Odi} & \textbf{Pun} & \textbf{Tam} & \textbf{Tel} & \textbf{Avg} \\
\midrule
\multicolumn{13}{l}{\textit{Recall@1 (\%)}} \\
multilingual-e5-large-instruct & 25.7 & 29.4 & 28.5 & 31.6 & 29.2 & 26.9 & 30.6 & 26.2 & 29.8 & 27.1 & 27.8 & 28.4 \\
BGE-M3 & 19.7 & 24.1 & 24.1 & 26.5 & 24.9 & 23.8 & 25.0 & 21.6 & 23.7 & 21.8 & 24.7 & 23.6 \\
Para-MPNet & -- & -- & 14.1 & 18.2 & -- & -- & 15.6 & -- & -- & -- & -- & 16.0 \\
indic-sentence-bert-nli & 13.1 & 16.4 & 16.3 & 18.4 & 16.7 & 14.4 & 15.6 & 11.8 & 18.1 & 15.3 & 16.7 & 15.7 \\
LaBSE & 6.6 & 15.1 & 17.7 & 19.2 & 16.2 & 12.2 & 15.5 & 13.9 & 15.9 & 15.8 & 15.8 & 14.9 \\
Para-XLM-R & -- & -- & 13.0 & 17.2 & -- & -- & 14.1 & -- & -- & -- & -- & 14.7 \\
indic-sentence-similarity-sbert & 11.8 & 13.6 & 13.4 & 14.4 & 13.7 & 11.3 & 13.0 & 9.1 & 14.4 & 12.4 & 12.7 & 12.7 \\
DistilUSE-Multi & -- & -- & 7.2 & 13.7 & -- & -- & 10.0 & -- & -- & -- & -- & 10.3 \\
\midrule
\multicolumn{13}{l}{\textit{MRR@10}} \\
multilingual-e5-large-instruct & 0.323 & 0.363 & 0.352 & 0.388 & 0.360 & 0.337 & 0.376 & 0.326 & 0.369 & 0.339 & 0.346 & 0.353 \\
BGE-M3 & 0.253 & 0.303 & 0.302 & 0.329 & 0.309 & 0.298 & 0.313 & 0.275 & 0.297 & 0.275 & 0.306 & 0.296 \\
Para-MPNet & -- & -- & 0.193 & 0.245 & -- & -- & 0.212 & -- & -- & -- & -- & 0.217 \\
indic-sentence-bert-nli & 0.184 & 0.222 & 0.222 & 0.245 & 0.225 & 0.197 & 0.214 & 0.167 & 0.240 & 0.209 & 0.225 & 0.214 \\
LaBSE & 0.092 & 0.198 & 0.227 & 0.244 & 0.210 & 0.161 & 0.202 & 0.181 & 0.205 & 0.204 & 0.203 & 0.193 \\
Para-XLM-R & -- & -- & 0.180 & 0.232 & -- & -- & 0.192 & -- & -- & -- & -- & 0.202 \\
indic-sentence-similarity-sbert & 0.163 & 0.183 & 0.181 & 0.194 & 0.185 & 0.157 & 0.176 & 0.129 & 0.192 & 0.171 & 0.173 & 0.173 \\
DistilUSE-Multi & -- & -- & 0.103 & 0.185 & -- & -- & 0.140 & -- & -- & -- & -- & 0.143 \\
\bottomrule
\end{tabular}
\caption{Cross-lingual instruction$\rightarrow$persona retrieval (T3 reverse) from Urdu to all target languages. Recall@1 (\%) and MRR@10 metrics shown for each source-target pair; averages computed over supported pairs only. Target language abbreviations: Ass=Assamese, Ben=Bengali, Guj=Gujarati, Hin=Hindi, Kan=Kannada, Mal=Malayalam, Mar=Marathi, Odi=Odia, Pun=Punjabi, Tam=Tamil, Tel=Telugu.}
\label{tab:t3_xling_reverse_urd}
\end{table*}
